# Supplementary material for: Re-using model results to determine materials properties: connector theory approach
Source: arXiv:1903.07930 ancillary file (2021-03-12)
Supplement: Supplementary file 1 [file suppmat.pdf]

# Supplemental Material for: Re-using model results to determine materials properties: connector theory approach

Marco Vanzini,<sup>1,2,3</sup> Ayoub Aouina,<sup>1,3</sup> Martin Panholzer,<sup>1,3,4</sup> Matteo Gatti,<sup>1,3,5</sup> and Lucia Reining<sup>1,3</sup>

<sup>1</sup>*Laboratoire des Solides Irradiés, École Polytechnique, CNRS,  
CEA/DRF/IRAMIS, Institut Polytechnique de Paris, F-91128 Palaiseau, France*

<sup>2</sup>*Theory and Simulation of Materials (THEOS), École Polytechnique Fédérale de Lausanne, CH-1015 Lausanne, Switzerland*

<sup>3</sup>*European Theoretical Spectroscopy Facility (ETSF)*

<sup>4</sup>*Johannes Kepler University Linz, Austria*

<sup>5</sup>*Synchrotron SOLEIL, L'Orme des Merisiers, Saint-Aubin, BP 48, F-91192 Gif-sur-Yvette, France*

(Dated: October 6, 2020)

This supplemental material contains a few intermediate mathematical steps to support the main equations of this work, and additional results for the interested reader.

## I. ONE-DIMENSIONAL ONE-ELECTRON PROBLEM

### A. Exact solution of the one-dimensional soft well

We consider in detail the potential discussed in the main text, which reads:

$$V(z) = \begin{cases} \frac{1}{2}m\omega_0^2(z + \frac{L}{2})^2 & z < -\frac{L}{2} \\ 0 & -\frac{L}{2} \leq z \leq \frac{L}{2} \\ \frac{1}{2}m\omega_0^2(z - \frac{L}{2})^2 & z > \frac{L}{2} \end{cases} \quad \begin{matrix} \text{(I)} \\ \text{(II)} \\ \text{(III),} \end{matrix}$$

with  $\omega_0$  and  $L$  real positive parameters: the larger  $\omega_0$ , the steeper the walls and the closer is the system to an infinite potential well. On the other hand, for vanishing  $L$ , the simple harmonic oscillator  $V(z) = \frac{1}{2}m\omega_0^2 z^2$  is recovered.

We are interested in the most general solution of the Schrödinger equation  $[-\frac{\hbar^2}{2m} \frac{d^2}{dz^2} + V(z)]\psi(z) = E\psi(z)$ . If we pass to the adimensional variable  $y \equiv z/L$  and consequently rescale the energy as  $E \rightarrow \varepsilon \equiv L^2 E$ , the relevant parameter for describing the Hamiltonian turns out to be  $\alpha \equiv 1/L^2 \omega_0$ . In fact, the Schrödinger equation for  $(\varepsilon, \psi(Ly))$  involves the potential  $V(y) = \frac{1}{\alpha^2} \frac{m}{2} (y \pm \frac{1}{2})^2$ . The Schrödinger equation is solved separately in each of the three regions (I), (II) and (III). Then, the solutions are glued by requiring the wavefunction and its first derivative to be continuous at the zone boundaries  $y = \pm \frac{1}{2}$ . The energy level  $\varepsilon$  is the solution to the equation connecting the different regions<sup>1</sup>:

$$\tan k = \frac{2kh}{k^2 - h^2}, \quad (1)$$

where  $k$  is the standard (region II) and  $h$  is a generalized (region I and III) wavevector, defined by:

$$k = \frac{1}{\hbar} \sqrt{2m\varepsilon} \quad h = \frac{2}{\sqrt{\alpha}} \sqrt{\frac{m}{\hbar}} \frac{\Gamma(-\frac{\alpha\varepsilon}{2\hbar} + \frac{3}{4})}{\Gamma(-\frac{\alpha\varepsilon}{2\hbar} + \frac{1}{4})},$$

with  $\Gamma$  the Gamma function. The two solutions of Eq. (1) are  $h_O = k \tan \frac{k}{2}$  and  $h_E = -k / \tan \frac{k}{2}$ , independent of

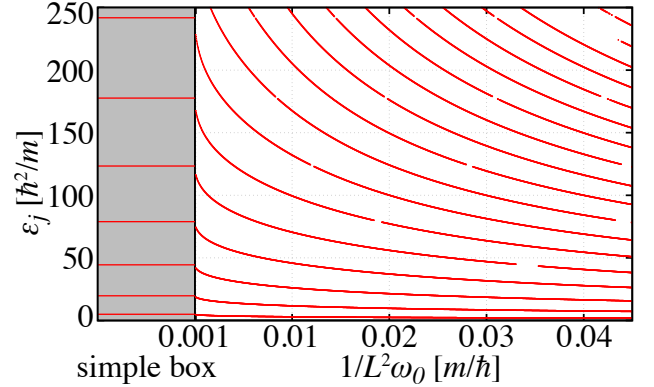

FIG. 1: In the main right panel, renormalized energy levels  $\varepsilon_j(\alpha)$ , in units of  $\hbar^2/m$ , as a function of  $\alpha = 1/L^2\omega_0$ , from  $L^2\omega_0 = 10000$  to  $L^2\omega_0 = 20$ , in units of  $m/\hbar$ . In the left panel, the renormalized energies  $\varepsilon_j^{\text{box}}$  of a simple box. Gaps in the energy levels are regions of the parameters for which the root-finder algorithm has problems.

$\alpha$  and with  $k = \frac{1}{\hbar} \sqrt{2m\varepsilon}$ . Using the definition of  $h$  yields two sets of discrete eigenvalues  $\{\varepsilon_O\}$  and  $\{\varepsilon_E\}$ . Ordering and labelling them with a single index  $j \geq 1$ , one obtains a series where  $\{\varepsilon_O\}$  correspond to odd and  $\{\varepsilon_E\}$  to even values of  $j$ .

In practice we determine the solutions  $E(j; \omega_0, L) = (1/L^2)\varepsilon_j(\alpha)$  for odd  $j$  numerically as the zeros of  $\sqrt{\frac{\varepsilon}{2\hbar}} \tan \sqrt{\frac{m\varepsilon}{2\hbar}} - \frac{1}{\sqrt{\alpha}} \frac{\Gamma(-\frac{\alpha\varepsilon}{2\hbar} + \frac{3}{4})}{\Gamma(-\frac{\alpha\varepsilon}{2\hbar} + \frac{1}{4})}$ , and analogously for even  $j$ . We have used the Ridder method<sup>2</sup> to find the roots. The result is shown in Fig. 1 for the first energy levels and different values of  $\alpha$ . For  $\alpha \rightarrow 0$ , we are back to the renormalized box eigenvalues  $\varepsilon_j^{\text{box}} = \frac{\hbar^2 \pi^2 j^2}{2m}$ , whose separation increases linearly with  $j$ . On the opposite side, where  $\alpha$  is larger, the eigenvalues are more and more evenly spaced, as for a simple oscillator. The gaps in the red lines of Fig. 1 indicate regions where the root-finder algorithm was not able to converge; this is not important for our illustration of the quality of the connector, but also stresses the gain that one may obtain from a more efficient approach, already in this very simple example.

## B. Perturbation expansion of the solution

In the limit of infinite frequency and finite  $L$ ,  $\alpha \rightarrow 0$  and the system becomes an infinite potential well with solutions  $\varepsilon_j \rightarrow \varepsilon_j^{\text{box}}$ : since  $\frac{\Gamma(\frac{3}{4})}{\Gamma(\frac{1}{4})} \equiv \gamma \approx 0.338$  is finite,  $h$  diverges to plus infinity and the right hand side of Eq. (1) goes to zero. Therefore, the eigenvalues are the solutions of the equation  $\tan \frac{\sqrt{2m\varepsilon}}{h} = 0$ , namely  $\frac{\sqrt{2m\varepsilon}}{h} = j\pi$ , that is  $\varepsilon_j = \frac{\hbar^2 \pi^2 j^2}{2m} \equiv \varepsilon_j^{\text{box}}$ ,  $j \geq 1$ .

The next order term is obtained by taking into account that  $\alpha$  is small but non zero, such that the  $1/\sqrt{\alpha}$  prefactor in  $h$  does not diverge, but the ratio of  $\Gamma$ -functions remains unchanged. This yields  $h \approx 2\gamma\sqrt{\frac{m}{h}}\frac{1}{\sqrt{\alpha}}$ . In this way, eq. (1) reads  $\tan \frac{\sqrt{2m\varepsilon}}{h} = -\frac{\sqrt{\alpha}}{\gamma}\sqrt{\frac{2\varepsilon}{h}}$ . Assuming  $\varepsilon = \varepsilon_j^{\text{box}} + \delta\varepsilon$ , with  $\delta\varepsilon/\varepsilon_j^{\text{box}} \ll 1$ , we obtain  $\delta\varepsilon = -\frac{2}{\gamma}\sqrt{\frac{\alpha h}{m}}\varepsilon_j^{\text{box}}$ . Therefore:

$$E^{\text{approx}}(j; \omega_0, L) = \frac{1}{L^2}\varepsilon_j^{\text{box}} \left[ 1 - \frac{2}{\gamma}\sqrt{\frac{h}{m}}\sqrt{\alpha(\omega_0, L)} \right]. \quad (2)$$

This approximate solution has of course a very small computational cost, compared to the exact one, and presents no numerical difficulties.

## C. The model system and the connector approach

We now try to reproduce the energy levels  $E(j; \omega_0, L)$  by connecting to a model system. We take as a model the simple infinite potential well of width  $\tilde{L}$ , *i.e.*,  $V_\infty(z) = V_0\theta(|z| - \frac{\tilde{L}}{2})$ , with  $V_0 \rightarrow \infty$ . Its energy spectrum is  $\mathcal{E}_{\tilde{j}}(\tilde{L}) = \frac{1}{L^2}\varepsilon_j^{\text{box}}$ . As one can set up a one-to-one correspondence between the energy levels of the real and the model system (e.g., by going to the infinite  $\omega_0$  limit), we can set  $\tilde{j} = j$  for simplicity.

As the observable  $O$  that we want to reproduce is the energy level  $E(j; \omega_0, L)$ , Eq. (3) of the main text reads:

$$E(j; \omega_0, L) = \mathcal{E}_j(L_{j\omega_0 L}^c) = \frac{\hbar^2 \pi^2 j^2}{2m(L_{j\omega_0 L}^c)^2},$$

and the exact connector reads:

$$L_{j\omega_0 L}^c = \frac{\hbar \pi j}{\sqrt{2mE(j; \omega_0, L)}}.$$

This would require calculation of the exact energy levels, which is what one wants to avoid. An approximate form of the connector is obtained from an expansion of the energy in both the real and the model systems around the same zeroth order, namely a box of length  $L$ . For the real system, this expansion is given by Eq. (2). The equivalent approximation for the model system consists

in an expansion in the parameter  $\tilde{L}$  around the box of length  $L$ , *i.e.*, around the same zeroth order as for the real system, to profit from error cancellations:

$$\begin{aligned} \mathcal{E}_j^{\text{approx}}(\tilde{L}) &= \mathcal{E}_j(L) + (\tilde{L} - L) \frac{d\mathcal{E}_j(L')}{dL'} \Big|_{L'=L} = \\ &= \mathcal{E}_j(L) \left[ 1 - 2\frac{\tilde{L}-L}{L} \right]. \end{aligned}$$

Now Eq. (4) of the main text,  $E^{\text{approx}}(j; \omega_0, L) = \mathcal{E}_j^{\text{approx}}(L_{j\omega_0 L}^{c, \text{approx}})$ , results in the following connector:

$$L_{\omega_0 L}^{c, \text{approx}} = L \left[ 1 + \frac{1}{\gamma} \sqrt{\frac{h}{m}} \frac{1}{\sqrt{L^2 \omega_0}} \right]. \quad (3)$$

This expression depends on  $L$  and  $\omega_0$  but not on  $j$ , as with the choice  $\tilde{j} = j$  the  $j^2$  dependence factorizes: this connector is transferable, *i.e.*, it could be calculated for one energy level and then used for all others. Also note that the difference between  $L^{c, \text{approx}}$  and  $L$  becomes smaller and smaller as  $\omega_0$  tends to infinity, namely as the real system approaches the model system itself.

Once the connector has been obtained, the energy levels are taken from the exact solution of the model system following Eq. (5) of the main text:

$$E^c(j; \omega_0, L) = \mathcal{E}_j(L_{\omega_0 L}^{c, \text{approx}}) = \frac{\mathcal{E}_j(L)}{\left[ 1 + \frac{1}{\gamma L} \sqrt{\frac{h}{m\omega_0}} \right]^2}. \quad (4)$$

Here, the first equality is what one would use in practice, when  $\mathcal{E}_j$  has been tabulated. There may also be cases, like the present example, where the entry in the table can be converted to a simple expression, for example a rescaling, as expressed by the second equality. This, however, is not a key requirement for the connector to be efficient. Note that Eq. (4) always leads to positive energies, contrary to the straightforward perturbation results Eq. (2) that become unphysical for large  $\alpha$ , as discussed and shown in Fig. 1 in the main text.

## II. BAND STRUCTURES USING APPROXIMATE TRANSFERABILITY

Here we give details of how to use COT to obtain a quick estimate of non-interacting or KS band structures, given the total potential  $V(\mathbf{r})$ . As model we take the HEG, where the band structure is simply the free electron parabola folded into the Brillouin zone, and its potential  $V^c$  is constant in space, with a value  $\mathcal{V}^c$  given with respect to the chemical potential. This potential plays the role of a connector. The connector potential is in principle different for each wavevector  $\mathbf{k}$ . Moreover, it should depend on the band. It may be difficult to find a one-to-one relation between the HEG bands and the bands of the real material. Therefore, we do not connect bands but spectral functions, by imposing the connector equality (Eq. (3) in the main text)

$$G_{\mathbf{K}\mathbf{K}}(\mathbf{k}, \omega; [V]) = \mathcal{G}_{\mathbf{k}\omega\mathbf{K}}(\mathcal{V}_{\mathbf{k}\omega\mathbf{K}}^c), \quad (5)$$

where  $G$  and  $\mathcal{G}$  are the KS Green's functions of the real material and the HEG, respectively, and  $\mathbf{K}$  are reciprocal lattice vectors. The HEG Green's function, which is diagonal in the reciprocal lattice vectors and therefore becomes a function of  $\mathbf{K}$ , is also a function of the value  $\mathcal{V}^c \in \mathbb{R}$  of the homogeneous potential,<sup>7</sup>

$$\mathcal{G}_{\mathbf{k}\omega\mathbf{K}}(\mathcal{V}^c) = \frac{1}{\omega - |\mathbf{k} + \mathbf{K}|^2/2 - \mathcal{V}^c}. \quad (6)$$

The spectral function is the imaginary part of the trace (here, a sum over  $\mathbf{K}$ ), therefore one could also ask for  $\sum_{\mathbf{K}} \text{Im} G_{\mathbf{K}\mathbf{K}}(\mathbf{k}, \omega; [V]) = \sum_{\mathbf{K}} \text{Im} \mathcal{G}_{\mathbf{k}\omega\mathbf{K}}(\mathcal{V}_{\mathbf{k}\omega}^c)$ , with a  $\mathbf{K}$ -independent connector potential  $\mathcal{V}_{\mathbf{k}\omega}^c$ . However, to invert this relation and select a unique answer would be much more cumbersome than to invert Eq. (5) to find  $\mathcal{V}^c$ , which simply yields

$$\mathcal{V}_{\mathbf{k}\omega\mathbf{K}}^c = \omega - \frac{|\mathbf{k} + \mathbf{K}|^2}{2} - \frac{1}{G_{\mathbf{K}\mathbf{K}}(\mathbf{k}, \omega; [V])}. \quad (7)$$

Here, the  $\omega$ -dependence is the translation of the fact that the connector is band-dependent, and that the bands of the HEG and the real system do not necessarily have a one-to-one correspondence. The exact connector in a point  $\mathbf{k}_0$  can be found by calculating  $G_{\mathbf{K}\mathbf{K}}(\mathbf{k}_0, \omega; [V])$ . To avoid diagonalizing the hamiltonian in every  $\mathbf{k}$ -point, our approximation is to neglect the  $\mathbf{k}$ -dependence of the connector, which is a hypothesis of transferability. Of course, applied directly to the band structure or spectral function, transferability would be a bad approximation, since it would read  $G_{\mathbf{K}\mathbf{K}}(\mathbf{k}, \omega; [V]) \approx G_{\mathbf{K}\mathbf{K}}(\mathbf{k}_0, \omega; [V])$  and therefore yield only flat bands. If we straightforwardly apply the connector scheme, instead, the approximation reads

$$\mathcal{V}_{\mathbf{k}\omega\mathbf{K}}^{c \text{ approx}} = \mathcal{V}_{\mathbf{k}_0\omega\mathbf{K}}^c, \quad (8)$$

and the final result is

$$G_{\mathbf{K}\mathbf{K}}^{c \text{ approx}}(\mathbf{k}, \omega; [V]) = \frac{1}{-\frac{|\mathbf{k} + \mathbf{K}|^2}{2} + \frac{|\mathbf{k}_0 + \mathbf{K}|^2}{2} + \frac{1}{G_{\mathbf{K}\mathbf{K}}(\mathbf{k}_0, \omega; [V])}}. \quad (9)$$

This corresponds to a diagonal approximation of the in principle exact Dyson equation that relates  $G_{\mathbf{k}}$  and  $G_{\mathbf{k}_0}$ . The result of this straightforward approximation is shown in the left panel of Fig. 2, for the case of solid cubic He<sup>3</sup>. The bands can be guessed, but the result is blurred. The reason is that the approximate connector violates an exact constraint: the poles of an exact Green's function are independent of the matrix element that is taken, since the matrix element only gives the intensity, and not the energy. Here, instead, we obtain different poles for every  $\mathbf{K}$ , which blurs the picture. To make the band structure emerge from the background, we make use of the exact constraint and of the fact that one can still identify bands approximately. This allows us to group poles that belong to one blurred band, and to choose the pole with the maximum intensity as the representative one. In practice, we carry out the identification of bands with the following

procedure that is applied independently at each  $\mathbf{k}$  (and therefore, does not necessitate any hypothesis about continuation of bands): (i) For each  $\mathbf{K}$ , we determine from the spectral function the lowest energy pole, which should in principle be the same for all  $\mathbf{K}$ . In practice, one finds a distribution. (ii) We first roughly gather together those poles that lie within ten standard deviations from the average position of the first pole. These poles appear with different intensities, whereas the true spectral function for non-interacting electrons should only show one, normalized, pole for the first band. Therefore, we sum the intensities of the approximate poles until the normalization is reached; these poles are assigned to the first band. The subsequent poles are assigned to the following band. Within the first group, the pole with maximum intensity is chosen to represent the band  $j = 1$ . (iii) The others are discarded, and the band counter moves on, from  $j = 1$  to  $j = 2$ . (iv) There may be  $\mathbf{K}$ 's for which the lowest pole is not visible, because it shows zero intensity. If the bands are not too dense, the next pole will lie outside of the standard deviation gathering. Also in this case, the counter moves to  $j = 2$ , but those poles will be re-considered. (v) The same procedure is applied to band  $j = 2$ , including as candidate poles the second lowest poles or, for the  $\mathbf{K}$  where (iv) was applied, the poles to be re-considered. The procedure then continues in the same way. Of course, it cannot restore the exact band structure and may fail for large unit cells where bands are very dense, or for materials very far from the HEG where no dominant poles may be identified, and it could certainly be refined. However, it has the advantage of being very simple and fast. Moreover, as can be seen from the example of cubic helium, it gives realistic results even for such an insulator with highly localized states, which is very far from a HEG or simple metal.

We do, however, wish to illustrate also the limits of this very simple approximation to COT. To this aim, Fig. 3 shows the equivalent results for solid hydrogen. The left panel shows the first principles band structure, which is very far from the HEG one, given also for comparison. The connector results in the right panel were obtained in the same way as for the example of helium. The main deviations from the HEG are well described, for example, the existence of a double band below 5 eV between L and A, or of the second band between  $\Gamma$  and M. At the same time, supplementing the information at  $\Gamma$  with the HEG yields a realistic idea of the dispersion of the bands, which would be completely flat otherwise. The connector band structure is instead less good between M and L, as one would expect for a path far from the reference point, i.e.  $\Gamma$ .

To improve, one can produce the exact results in a few more  $\mathbf{k}$ -points, assuming transferability of the connector over a part of the Brillouin zone only. In the next section, we will instead discuss how results could be improved by improving the model, which is more pertinent in the spirit of COT.

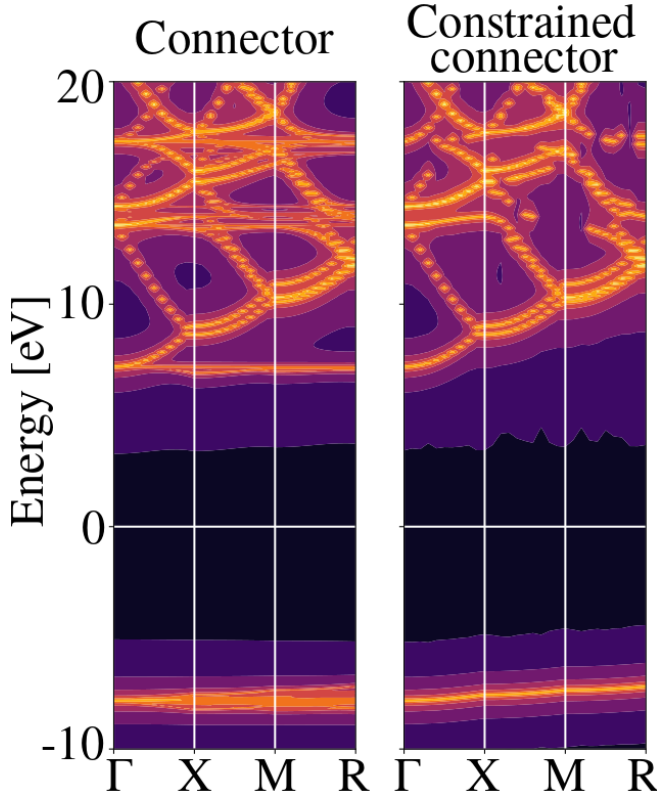

FIG. 2: Band structure of cubic helium, connector without constraints (left) and connector with exact constraints (right).

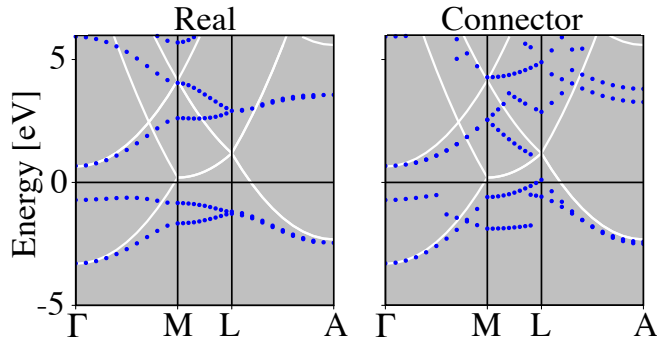

FIG. 3: Band structure of solid hydrogen, reference result (left) and connector with exact constraints (right), in blue. In white, HEG folded into the Brillouin zone of hydrogen and attached to the first valence band at  $\Gamma$ .

### A. Computational details

The reference band structures of cubic helium<sup>3</sup> and hexagonal hydrogen<sup>4</sup> have been obtained from the diagonalization of the KS-LDA Hamiltonian employing local norm-conserving pseudopotentials. The size of the Hamiltonian in reciprocal space was 5.1 Ha and 3.4 Ha for He and H, respectively.

### III. OUTLOOK: IMPROVED MODEL SYSTEM

One important question is whether COT approximations can be made systematically better. This is trivially the case when the chosen approximation can be systematically improved, as it is, e.g., the case for converging perturbation series, or, in the example of the band structure calculation, by using more than one  $\mathbf{k}_0$ . However, as pointed out in the main text, the benefit from using COT will be larger when instead the model is improved. This is possible in many cases, and sometimes straightforward. In particular, when  $Q^R$  is a function that can be decomposed into components such as Fourier components, the model function  $Q^c$  may be the lowest component (e.g. a constant) in the simplest case, or it may contain a very limited number of higher components. The COT procedure will work as before, although the connector will be a vector instead of a scalar, and for an increasing number of components, the COT approximation will tend to the exact result. Of course, the calculation of the model will become more cumbersome, and with an increasing number of components it will be more difficult to tabulate the results over the necessary range of parameters. Nevertheless, improving the model by going some way beyond the simplest possible one may be of large practical usefulness and within reach with today's computer and storage facilities.

To make this discussion more tangible, let us take the example of the band structure calculation. As above, we start by considering the HEG as model system. In this model the potential  $V_{\mathbf{K}\mathbf{K}}^c$  only has Fourier components  $\mathbf{K} = \mathbf{K}'$ , so we have  $\mathcal{V}^c \equiv V_{\mathbf{K}\mathbf{K}} = V_{00}$ . As an extended model, we could allow more Fourier components, for example, we could limit  $\mathbf{K}$  and  $\mathbf{K}'$  to lie in the same shell (i.e., to have the same length). Then, the model Green's function changes from (6) and becomes

$$\mathcal{G}_{\mathbf{k}\omega\mathbf{K}\mathbf{K}'}(\mathcal{V}^c) = \left( \delta_{\mathbf{K}\mathbf{K}'} \left( \omega - \frac{|\mathbf{k} + \mathbf{K}|^2}{2} \right) - \mathcal{V}_{\mathbf{K}\mathbf{K}'}^c \right)_{\mathbf{K}\mathbf{K}'}^{-1}, \quad (10)$$

in each shell separately; note that  $\mathcal{V}^c$  is now a matrix. This matrix can be determined uniquely by asking for  $G_{\mathbf{K}\mathbf{K}'}(\mathbf{k}, \omega)$  to equal  $\mathcal{G}_{\mathbf{k}\omega\mathbf{K}\mathbf{K}'}$ , again for each shell separately, which yields the exact connector matrix

$$\mathcal{V}_{\mathbf{K}\mathbf{K}'}^c = \delta_{\mathbf{K}\mathbf{K}'} \left( \omega - \frac{|\mathbf{k} + \mathbf{K}|^2}{2} \right) - G_{\mathbf{K}\mathbf{K}'}^{-1, shell}(\mathbf{k}, \omega), \quad (11)$$

where  $G_{\mathbf{K}\mathbf{K}'}^{-1, shell}(\mathbf{k}, \omega)$  is the inverse of a block of the full Green's function that lies within a shell. If one would go further and group more and more shells,  $\mathcal{V}^c$  would go to the exact potential, within increasing parts of Fourier space.

One can then make the same approximation as before, i.e. suppose transferability,

$$\mathcal{V}_{\mathbf{k}\omega\mathbf{K}\mathbf{K}'}^c \approx \mathcal{V}_{\Gamma\omega\mathbf{K}\mathbf{K}'}^c. \quad (12)$$

Since the connector potential tends to the exact potential for increasing size of the matrix, and since the exact

potential does not depend on  $\mathbf{k}$ , this approximation becomes exact in that limit. In other words, this example shows how systematic improvement of the model leads to systematically improved COT results. Other ways to build a model that contains more information than the HEG are possible, and it is beyond the scope of the present work to elucidate which will be the most promising route to take in practice.

#### IV. FIRST-ORDER CONNECTOR FOR DENSITY FUNCTIONALS

In this section, we show how one can design a first-order connector for the KS xc potential, and we illustrate its use and performance taking as target a known, nonlocal functional.

##### A. Designing a connector

Here we want to design a first-order connector that allows us to use the knowledge of the xc potential of the HEG to approximate the exact functional. To do so, we start from the exact connection:

$$v_{xc}(\mathbf{r}_1, [n]) = v_{xc}^h(n_{h\mathbf{r}_1}^c), \quad (13)$$

where  $n_{h\mathbf{r}_1}^c$  is the unknown homogeneous density that yields the exact value of the xc potential  $v_{xc}(\mathbf{r}_1, [n])$  at position  $\mathbf{r}_1$ , when plugged in the xc potential of the HEG  $v_{xc}^h(n_h)$ . In order to get an approximate connector  $n_{h\mathbf{r}_1}^{c,approx}$ , we expand both sides of Eq. (13) to first order around a fixed homogeneous density  $n_0$ . This yields:

$$\int d\mathbf{r}_2 (n(\mathbf{r}_2) - n_0) f_{xc}(|\mathbf{r}_1 - \mathbf{r}_2|; n_0) = (n_{h\mathbf{r}_1}^{c,approx} - n_0) f_{xc}^h(n_0), \quad (14)$$

where  $f_{xc}(|\mathbf{r}_1 - \mathbf{r}_2|; n_0) = \delta v_{xc}(\mathbf{r}_1, [n]) / \delta n(\mathbf{r}_2)|_{n=n_0}$  is the static nonlocal xc kernel of the HEG with density  $n_0$ , and  $f_{xc}^h(n_0) = dv_{xc}^h(n_h) / dn_h|_{n_h=n_0}$  is its limit of zero wavevector, which corresponds to the case where variations are restricted such that the density remains homogeneous, i.e., we remain within the parameter space given by the model. The zeroth order term  $v_{xc}^h(n_0)$ , that appears in both sides, is simplified. Finally, inverting the equation we get:

$$n_{h\mathbf{r}_1}^{c,approx}([n]) = \frac{1}{f_{xc}^h(n_0)} \int d\mathbf{r}_2 n(\mathbf{r}_2) f_{xc}(|\mathbf{r}_1 - \mathbf{r}_2|; n_0). \quad (15)$$

This is the first-order connector discussed in the main text. Note that for slowly varying density  $n$  one can pull  $n$  out of the integral, which leads to the correct limiting case, i.e. the LDA.

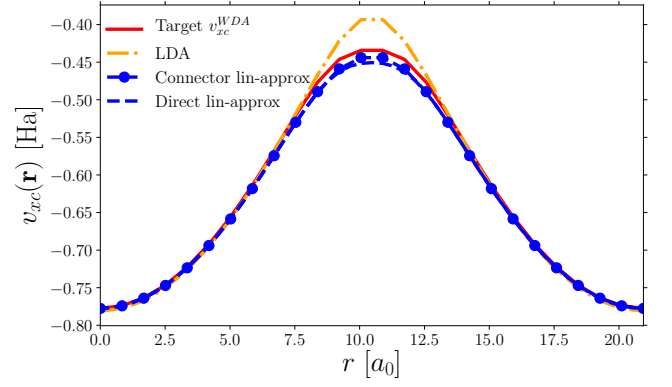

FIG. 4: Comparison between the target WDA xc potential (red line) and different approximations: LDA (yellow line), direct linear approximation (green line) and using the connector (blue line) for slowly varying density. In this case  $n(\mathbf{r}) = A \cos(\mathbf{a} \cdot \mathbf{r}) + B$ , where  $a = 0.3 a_0^{-1}$ ,  $n_{max} = 0.3776 a_0^{-3}$  and  $n_{min} = 0.0402 a_0^{-3}$ .

##### B. Weighted density approximation

To highlight the features of the connector designed in the previous section, as discussed in the main text we choose a known functional as target for the connector approach. Our example is the functional given by the weighted density approximation (WDA)<sup>5</sup> that reads:

$$E_{xc}^{WDA}[n] = \int d\mathbf{r} d\mathbf{r}' \frac{n(\mathbf{r})n(\mathbf{r}')}{2|\mathbf{r}' - \mathbf{r}|} C(\tilde{n}(\mathbf{r}, \mathbf{r}')) \left(1 - e^{-\frac{\lambda(\tilde{n}(\mathbf{r}, \mathbf{r}'))}{|\mathbf{r}' - \mathbf{r}|^5}}\right),$$

where  $\tilde{n}(\mathbf{r}, \mathbf{r}') = [n(\mathbf{r}) + n(\mathbf{r}')]/2$ . To determine the parameters  $C$  and  $\lambda$  we impose that  $E_{xc}$  is exact in the HEG, and fulfills the sum rule  $\int d\mathbf{r}' n_{xc}(\mathbf{r}, \mathbf{r}' - \mathbf{r}) = -1$ . From these two constraints we get:

$$\lambda(n) = \left( \frac{-3\Gamma(\frac{3}{5})}{4\Gamma(\frac{2}{5}) \varepsilon_{xc}(n)} \right)^5 \quad \text{and} \quad C(n) = \frac{-3/4\pi}{\Gamma(\frac{2}{5}) (\lambda(n))^{\frac{3}{5}} n},$$

where  $\varepsilon_{xc}(n)$  is the exact xc energy per particle of the HEG, whose correlation part we take from the parameterization of Chachiyo<sup>6</sup>. To get the target xc potential we perform the functional derivative of the xc energy,  $\frac{\delta E_{xc}[n]}{\delta n(\mathbf{r}_1)}$ . It yields :

$$\begin{aligned} v_{xc}^{WDA}(\mathbf{r}_1, [n]) = & \frac{1}{2} \left[ \int d\mathbf{r}' \frac{2n(\mathbf{r}')}{|\mathbf{r}' - \mathbf{r}_1|} C(\tilde{n}(\mathbf{r}', \mathbf{r}_1)) \left(1 - e^{-\frac{\lambda(\tilde{n}(\mathbf{r}', \mathbf{r}_1))}{|\mathbf{r}' - \mathbf{r}_1|^5}}\right) \right. \\ & + n(\mathbf{r}_1) \int d\mathbf{r}' \frac{n(\mathbf{r}')}{|\mathbf{r}' - \mathbf{r}_1|} C'(\tilde{n}(\mathbf{r}', \mathbf{r}_1)) \left(1 - e^{-\frac{\lambda(\tilde{n}(\mathbf{r}', \mathbf{r}_1))}{|\mathbf{r}' - \mathbf{r}_1|^5}}\right) \\ & \left. + n(\mathbf{r}_1) \int d\mathbf{r}' \frac{n(\mathbf{r}')}{|\mathbf{r}' - \mathbf{r}_1|^6} C(\tilde{n}(\mathbf{r}', \mathbf{r}_1)) \lambda'(\tilde{n}(\mathbf{r}', \mathbf{r}_1)) e^{-\frac{\lambda(\tilde{n}(\mathbf{r}', \mathbf{r}_1))}{|\mathbf{r}' - \mathbf{r}_1|^5}} \right]. \end{aligned}$$

Now, from the knowledge of the xc potential of the HEG, we want to approximate the functional  $v_{xc}(\mathbf{r}_1, [n])$  using

the connector approach. From Eq. (15) the main ingredient that we need in order to calculate a first-order connector is  $f_{xc}(|\mathbf{r}_1 - \mathbf{r}_2|; n_0)$ . In order to simulate a realistic situation,  $f_{xc}$  has to be consistent with the  $v_{xc}$  that one is heading for. Therefore we cannot use expressions for  $f_{xc}$  given in the literature, but we have to calculate the functional derivative of our target xc potential, and evaluate it at the constant density  $n_0$ . The resulting  $f_{xc}^{\text{WDA}}$  can be expressed as the sum of six terms,  $f_{xc}^{\text{WDA}}(|\mathbf{r}_1 - \mathbf{r}_2|; n_0) = \sum_{i=1}^6 f_i$ , with:

$$\begin{aligned} f_1 &= \left[ C(n_0) + n_0 C'(n_0) + \frac{1}{4} n_0^2 C''(n_0) \right] \frac{1 - e^{\frac{-\lambda(n_0)}{|\mathbf{r}_1 - \mathbf{r}_2|^5}}}{|\mathbf{r}_1 - \mathbf{r}_2|} \\ f_2 &= 2\pi\Gamma\left(\frac{3}{5}\right) (\lambda(n_0))^{\frac{2}{5}} \left[ n_0 C'(n_0) + \frac{1}{4} n_0^2 C''(n_0) \right] \delta(\mathbf{r}_1 - \mathbf{r}_2) \\ f_3 &= \left[ n_0 C(n_0) \lambda'(n_0) + \frac{1}{2} n_0^2 C'(n_0) \lambda'(n_0) + \frac{1}{4} n_0^2 C(n_0) \lambda''(n_0) \right] \\ &\quad \times \frac{e^{\frac{-\lambda(n_0)}{|\mathbf{r}_1 - \mathbf{r}_2|^5}}}{|\mathbf{r}_1 - \mathbf{r}_2|^6} \\ f_4 &= \frac{4\pi\Gamma\left(\frac{3}{5}\right)}{5(\lambda(n_0))^{\frac{3}{5}}} \left[ n_0 C(n_0) \lambda'(n_0) + \frac{1}{2} n_0^2 C'(n_0) \lambda'(n_0) \right. \end{aligned}$$

$$\left. + \frac{1}{4} n_0^2 C(n_0) \lambda''(n_0) \right] \delta(\mathbf{r}_1 - \mathbf{r}_2)$$

$$f_5 = -\frac{1}{4} n_0^2 C(n_0) (\lambda'(n_0))^2 \frac{e^{\frac{-\lambda(n_0)}{|\mathbf{r}_1 - \mathbf{r}_2|^5}}}{|\mathbf{r}_1 - \mathbf{r}_2|^{11}}$$

$$f_6 = -\frac{\pi\Gamma\left(\frac{8}{5}\right)}{5(\lambda(n_0))^{\frac{8}{5}}} n_0^2 C(n_0) (\lambda'(n_0))^2 \delta(\mathbf{r}_1 - \mathbf{r}_2)$$

This xc kernel  $f_{xc}^{\text{WDA}}(|\mathbf{r}_1 - \mathbf{r}_2|; n_0)$  is now used in Eq. (15) to get an approximate connector, which finally determines how to use the HEG results to simulate a real system, *via*

$$v_{xc}^c(\mathbf{r}_1, [n]) = v_{xc}^h(n^h = n_{hr1}^{c,approx}([n])). \quad (16)$$

Results for a density with an amplitude of variation that is typical for a rare gas solid are given in Fig. 3 of the main text. Here, we show in Fig. 4 for a slowly varying density, i.e. smaller  $\mathbf{a}$ , the xc potential obtained from the connector and we compare it to the other approaches. In particular, the figure shows that the connector result tends to the LDA, which itself tends to the exact result, when the density approaches the homogeneous limit.

<sup>1</sup> F. Balestri, *Alcuni aspetti della quantizzazione dell'oscillatore armonico*, Master thesis, Università di Bologna (2013).

<sup>2</sup> C. Ridders, IEEE Transactions on Circuits and Systems **26**, 979 (1979).

<sup>3</sup> A. F. Schuch and R. L. Mills, Phys. Rev. Lett. **6**, 596 (1961).

<sup>4</sup> S. N. Ishmaev, I. P. Sadikov, A. A. Chernyshev, B. A. Vin-

dryevsky, V. A. Sukhoparov, A. S. Telepnev, and G. V. Kobelyev, JETP **57**, 228 (1983).

<sup>5</sup> O. Gunnarsson and R. Jones, Phys. Scr. **21**, 394 (1980).

<sup>6</sup> T. Chachiyo, The Journal of Chemical Physics **145**, 021101 (2016).

<sup>7</sup> We use atomic units hereafter.
